# Supplementary material for: The Faintest, Extremely Variable X-ray Tidal Disruption Event from a Supermassive Black Hole Binary?
Source: arXiv:2511.21243 source file (2025-11-26)
Supplement: Supplementary file 1 [file Supplemental.pdf]

## Supplemental Information

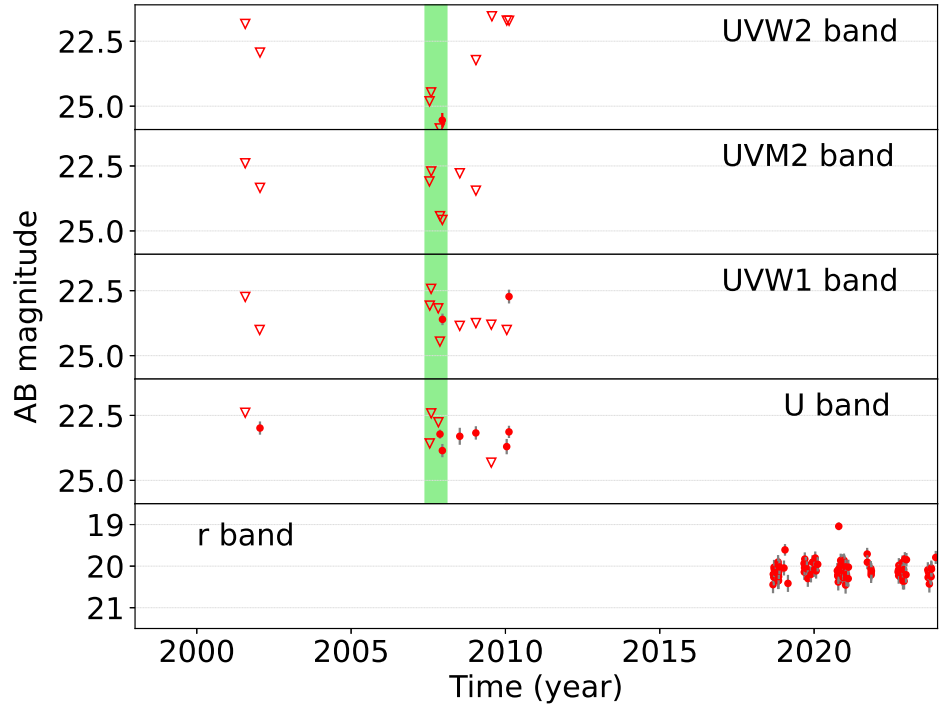

Figure S1: **Optical/UV light curves of XID 935.** From top to bottom, the bands are rest-frame UVW2, UVM2, UVW1, U, and r bands, respectively. For UVW2, UVM2, UVW1, and U bands, the Swift/UVOT data are green-shaded; outside the shaded region are the XMM-Newton/OM data. The r-band data are from the ZTF. Error bars correspond to  $1\text{-}\sigma$  uncertainties. Triangles are 90%-confidence-level upper limits.

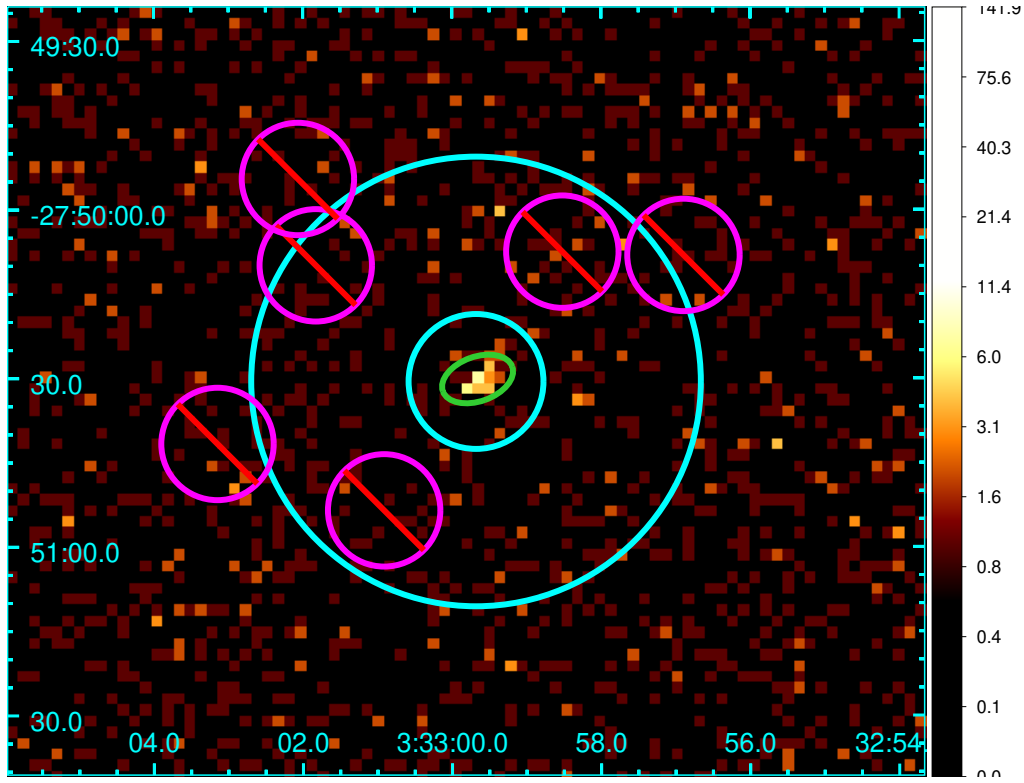

Figure S2: **Extraction region for XID 935 in the CDF-S.** The green ellipse is the source region. The cyan annulus is the background region, with 6 adjacent sources masked using magenta circles.

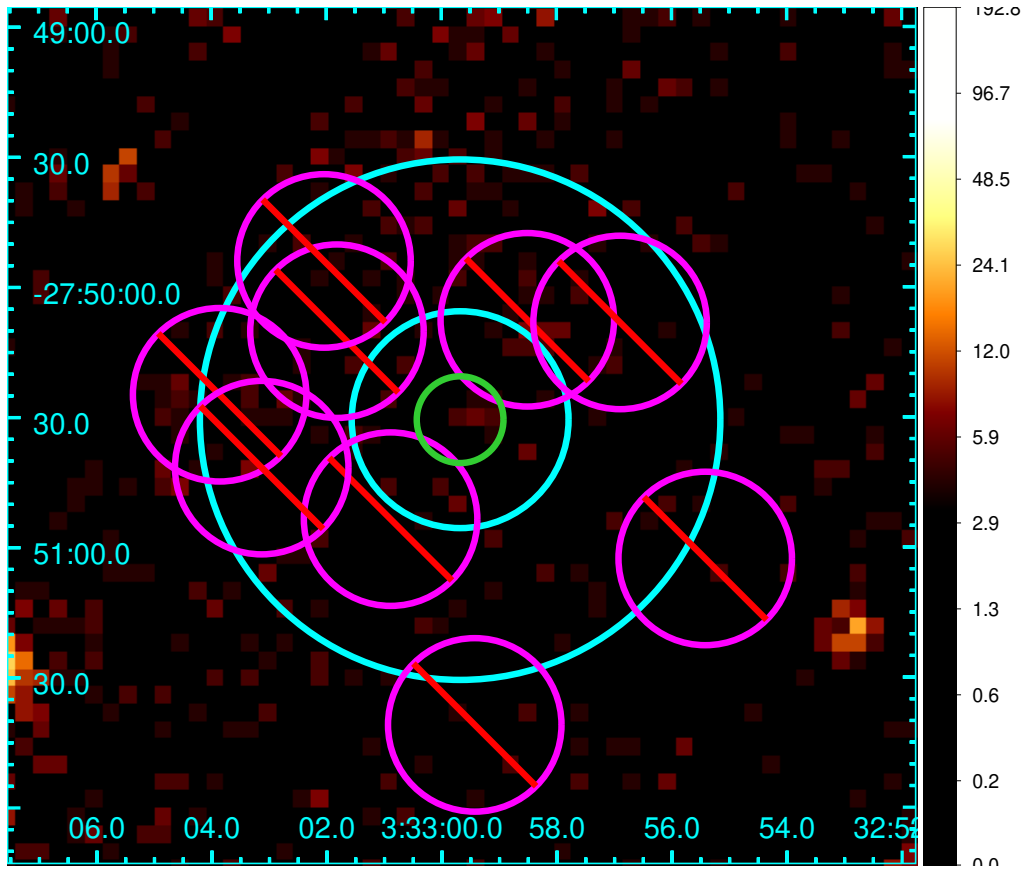

Figure S3: **Extraction region for XID 935 in the XMM-CDFS.** The green circle is the source region, and the cyan annulus is the background region, with 9 adjacent sources masked using magenta circles.

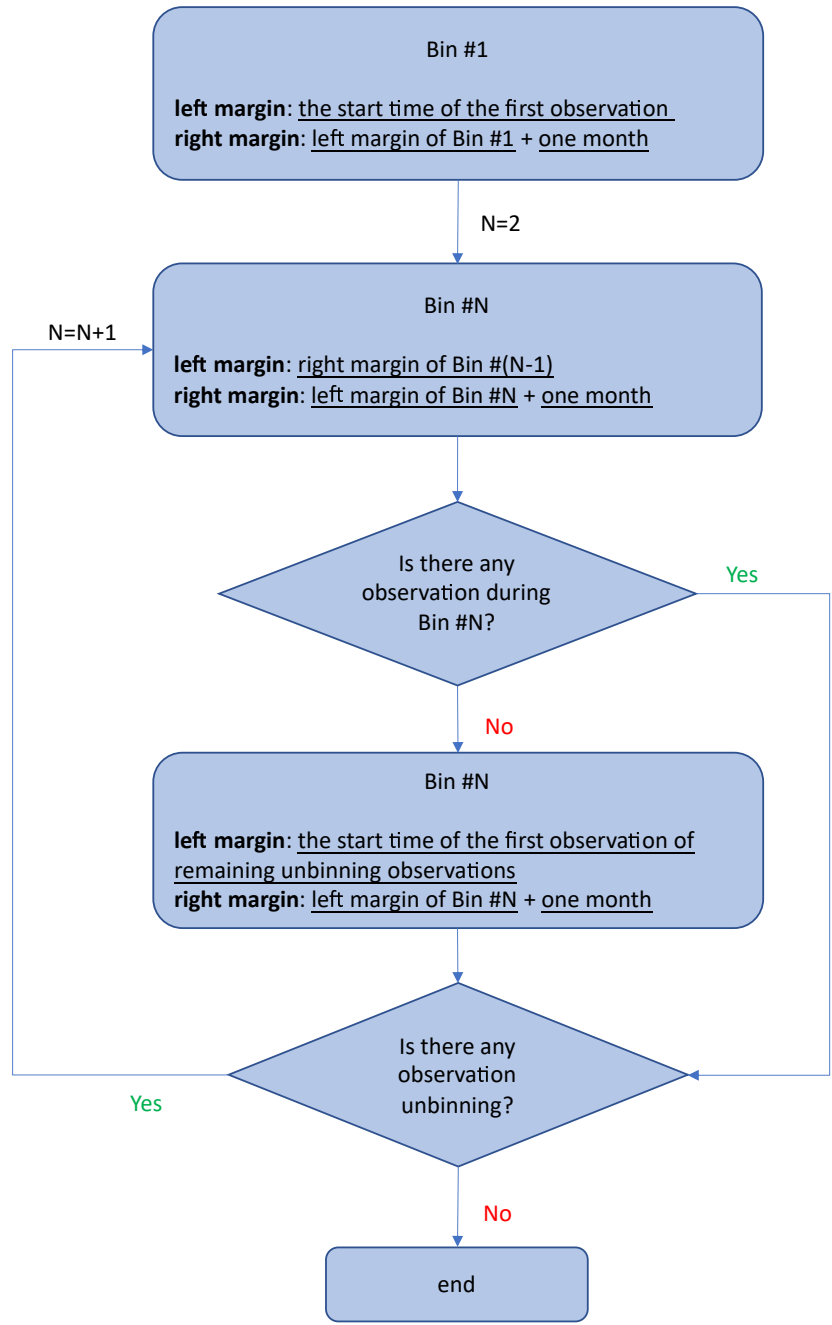

Figure S4: Month-bin flow diagram.

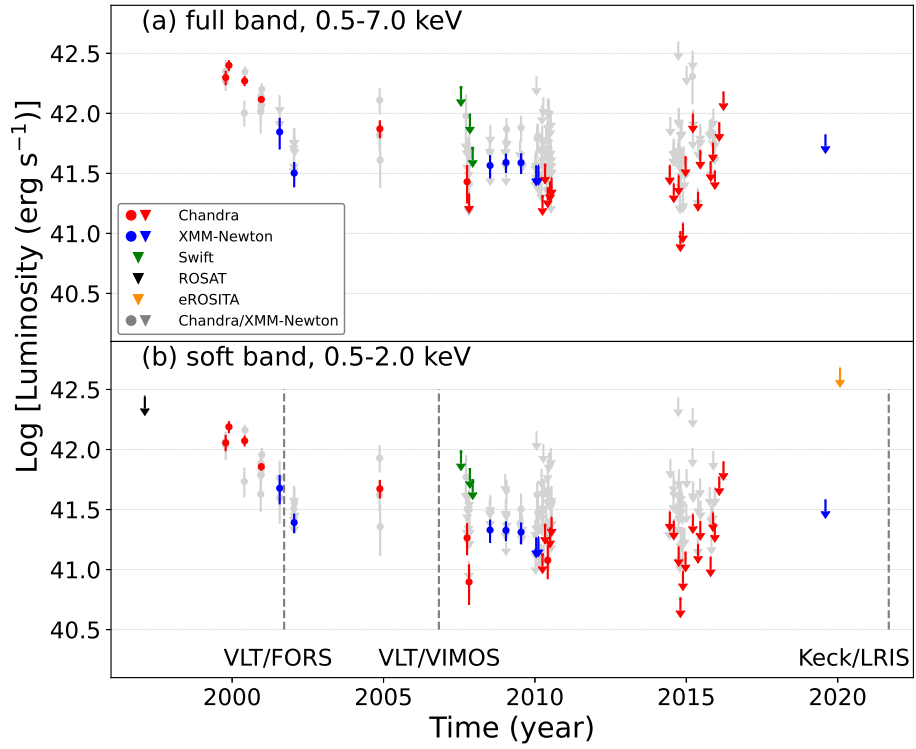

Figure S5: **Month-bin X-ray light curves of XID 935.** (a) Light curve in the rest-frame 0.5–7.0 keV band (full band, containing  $768.9 \pm 43.3$  and  $905.0 \pm 84.0$  Chandra and XMM-Newton net counts, respectively). (b) Light curve in the rest-frame 0.5–2.0 keV band (soft band, containing  $595.9 \pm 28.5$  and  $680.7 \pm 62.6$  Chandra and XMM-Newton net counts, respectively). Red, dark blue, green, black, and orange data are from Chandra, XMM-Newton, Swift, ROSAT, and eROSITA, respectively. Grey data represent individual observations of Chandra and XMM-Newton. Arrows indicate 90%-confidence-level upper limits. Dashed lines denote the observation times of optical spectra.

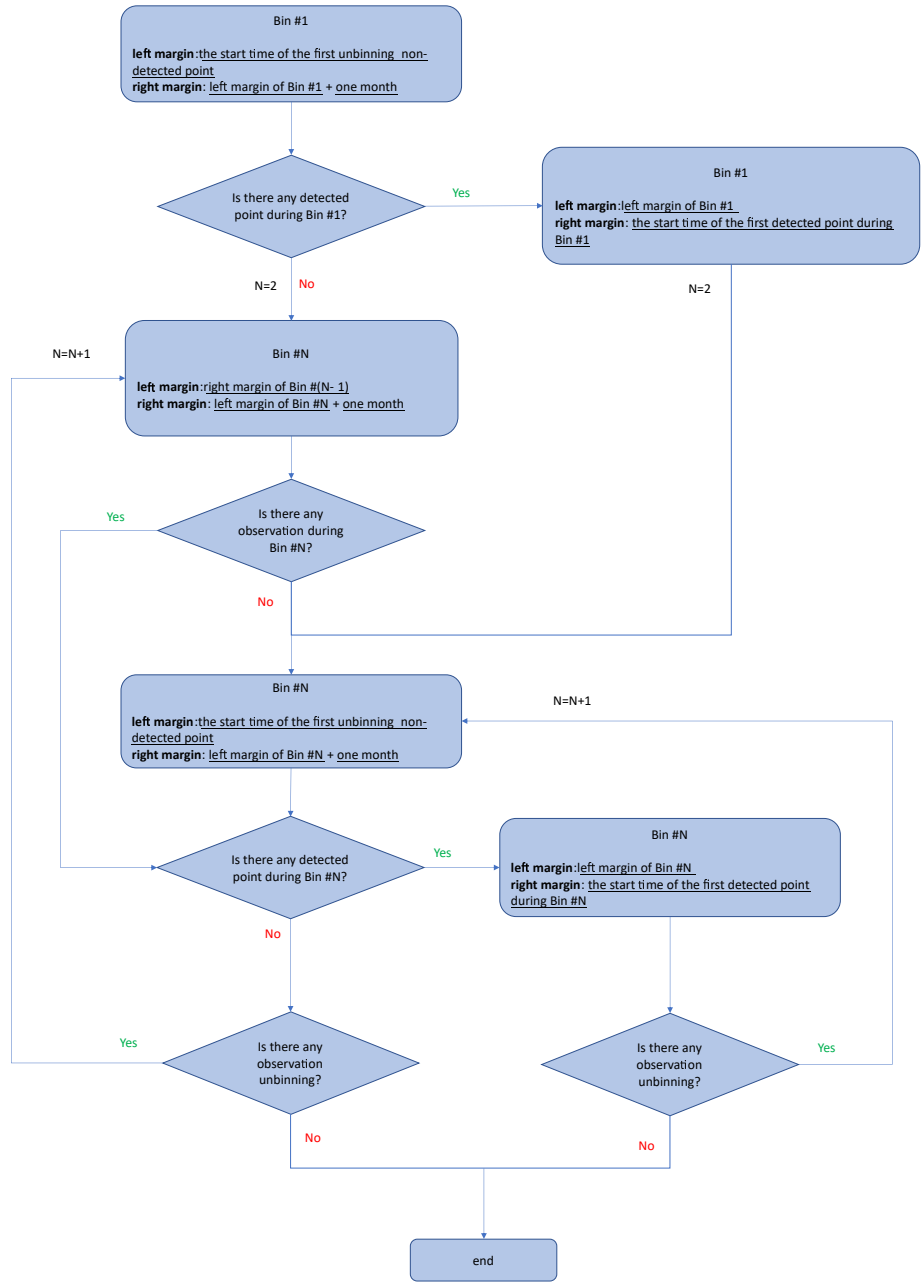

Figure S6: Adaptive-bin flow diagram.

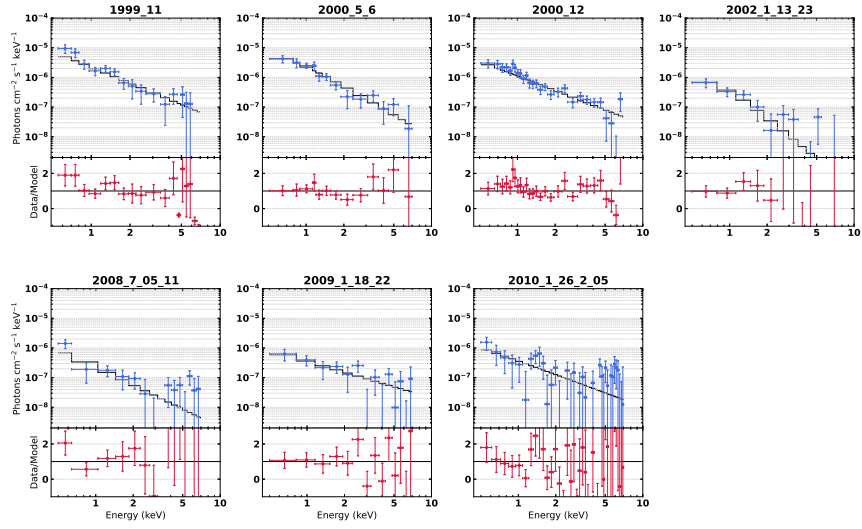

Figure S7: **X-ray spectra of XID 935.** Each panel displays the fitted spectrum and data-to-model ratio for time bins with net counts exceeding 60.

```

1 from scipy.special import xlogy # returns x * log(y), and return 0 if x=0 no matter y
2 import numpy as np
3 from scipy.stats import norm
4
5 src_cts = value1 # total counts in source region
6 bkg_cts = value2 # total counts in background region
7 src_backscal = value3 # area of source region
8 bkg_backscal = value4 # area of background region
9
10 def LRT(Src, Bkg, BkgScale=None):
11     if BkgScale is None:
12         try:
13             net = Src - Bkg
14             neglnLR = Bkg - Src + xlogy(Src, Src / Bkg)
15         except ZeroDivisionError:
16             return np.nan, np.nan
17     else:
18         net = Src - Bkg / BkgScale
19         tot = Src + Bkg
20         neglnLR = xlogy(Src, Src*(1 + BkgScale)/tot) + xlogy(Bkg, Bkg*(1 + BkgScale)/(BkgScale * tot))
21
22     Z = np.where(net < 0, -np.sqrt(2 * neglnLR), np.sqrt(2 * neglnLR))
23     return Z, norm.sf(Z)
24
25 Z, P_value = LRT(src_cts, bkg_cts, bkg_backscal / src_backscal)
26 print(Z) # Z in sigma units
27 print(P_value)

```

Listing S1: LRT Python code

Table S1: Chandra and XMM-Newton Observations

| Observation ID | Date       | One-month Bin |                 | Adaptive Bin |               |
|----------------|------------|---------------|-----------------|--------------|---------------|
|                |            | Total Exp.    | Bin Name        | Total Exp.   | Bin Name      |
| Chandra        | XMM-Newton | (ks)          |                 | (ks)         |               |
| 581            | 1999/10/14 | 68.5          | 1999_10         | 68.5         | 1999_10       |
| 1431-0         | 1999/10/15 |               |                 |              |               |
| 1431-1         | 1999/11/23 | 93.2          | 1999_11         | 93.2         | 1999_11       |
| 441            | 2000/5/27  | 181.1         | 2000_5_6        | 181.1        | 2000_5_6      |
| 582            | 2000/6/3   |               |                 |              |               |
| 2406           | 2000/12/10 | 631.4         | 2000_12         | 631.4        | 2000_12       |
| 2405           | 2000/12/11 |               |                 |              |               |
| 2312           | 2000/12/13 |               |                 |              |               |
| 1672           | 2000/12/16 |               |                 |              |               |
| 2409           | 2000/12/19 |               |                 |              |               |
| 2313           | 2000/12/21 |               |                 |              |               |
| 2239           | 2000/12/23 |               |                 |              |               |
| 0108060401     | 2001/7/27  | 33.2          | 2001_7          | 33.2         | 2001_7        |
| 0108060501     | 2001/7/27  |               |                 |              |               |
| 0108060601     | 2002/1/13  | 198.0         | 2002_1          | 198.0        | 2002_1_13_23  |
| 0108060701     | 2002/1/14  |               |                 |              |               |
| 0108061801     | 2002/1/16  |               |                 |              |               |
| 0108061901     | 2002/1/17  |               |                 |              |               |
| 0108062101     | 2002/1/20  |               |                 |              |               |
| 0108062301     | 2002/1/23  |               |                 |              |               |
| 5021           | 2004/11/13 | 241.3         | 2004_11         | 241.3        | 2004_11       |
| 5022           | 2004/11/15 |               |                 |              |               |
| 6164           | 2004/11/20 |               |                 |              |               |
| 8591           | 2007/9/20  | 359.8         | 2007_9_20_10_19 | 45.4         | 2007_9_20     |
| 9593           | 2007/9/22  |               |                 | 43.4         | 2007_9_22     |
| 9718           | 2007/10/3  |               |                 | 618.4        | 2007_10_03_30 |
| 8593           | 2007/10/6  |               |                 |              |               |
| 8597           | 2007/10/17 |               |                 |              |               |
| 8595           | 2007/10/19 |               |                 |              |               |

Table S1 continued from previous page

|       |            |            |       |                  |       |                |
|-------|------------|------------|-------|------------------|-------|----------------|
| 8592  |            | 2007/10/22 | 600.1 | 2007_10_22_11_04 |       |                |
| 8596  |            | 2007/10/24 |       |                  |       |                |
| 9575  |            | 2007/10/27 |       |                  |       |                |
| 9578  |            | 2007/10/30 |       |                  |       |                |
| 8594  |            | 2007/11/1  |       |                  | 140.9 | 2007_11_01     |
| 9596  |            | 2007/11/4  |       |                  | 111.8 | 2007_11_04     |
|       | 0555780101 | 2008/7/5   | 378.9 | 2008_7           | 378.9 | 2008_7_05_11   |
|       | 0555780201 | 2008/7/7   |       |                  |       |                |
|       | 0555780301 | 2008/7/9   |       |                  |       |                |
|       | 0555780401 | 2008/7/11  |       |                  |       |                |
|       | 0555780501 | 2009/1/6   | 593.3 | 2009_1_06_24     | 313.3 | 2009_1_06_16   |
|       | 0555780601 | 2009/1/10  |       |                  |       |                |
|       | 0555780701 | 2009/1/12  |       |                  |       |                |
|       | 0555780801 | 2009/1/16  |       |                  |       |                |
|       | 0555780901 | 2009/1/18  |       |                  | 184.5 | 2009_1_18_22   |
|       | 0555781001 | 2009/1/22  |       |                  |       |                |
|       | 0555782301 | 2009/1/24  |       |                  | 95.5  | 2009_1_24      |
|       | 0604960301 | 2009/7/5   | 375.0 | 2009_7_05_29     | 91.0  | 2009_7_05      |
|       | 0604960201 | 2009/7/17  |       |                  | 88.6  | 2009_7_17      |
|       | 0604960101 | 2009/7/27  |       |                  | 195.4 | 2009_7_27_29   |
|       | 0604960401 | 2009/7/29  |       |                  |       |                |
|       | 0604961101 | 2010/1/4   | 374.8 | 2010_1_04_26     | 283.5 | 2010_1_04_19   |
|       | 0604961201 | 2010/1/8   |       |                  |       |                |
|       | 0604960701 | 2010/1/12  |       |                  |       |                |
|       | 0604960501 | 2010/1/18  |       |                  |       |                |
|       | 0604961301 | 2010/1/19  |       |                  |       |                |
|       | 0604960601 | 2010/1/26  |       |                  | 172.9 | 2010_1_26_2_05 |
|       | 0604960801 | 2010/2/5   | 329.9 | 2010_2_05_17     |       |                |
|       | 0604960901 | 2010/2/11  |       |                  | 248.4 | 2010_2_11_17   |
|       | 0604961001 | 2010/2/13  |       |                  |       |                |
|       | 0604961801 | 2010/2/17  |       |                  |       |                |
| 12043 |            | 2010/3/18  | 694.0 | 2010_3_18_4_16   | 874.5 | 2010_3_18_5_17 |
| 12123 |            | 2010/3/21  |       |                  |       |                |
| 12044 |            | 2010/3/23  |       |                  |       |                |

Table S1 continued from previous page

|       |           |       |                |       |                 |
|-------|-----------|-------|----------------|-------|-----------------|
| 12128 | 2010/3/27 |       |                |       |                 |
| 12045 | 2010/3/28 |       |                |       |                 |
| 12129 | 2010/4/3  |       |                |       |                 |
| 12135 | 2010/4/6  |       |                |       |                 |
| 12046 | 2010/4/8  |       |                |       |                 |
| 12047 | 2010/4/12 |       |                |       |                 |
| 12137 | 2010/4/16 |       |                |       |                 |
| 12138 | 2010/4/18 | 180.5 | 2010_4_18_5_17 |       |                 |
| 12055 | 2010/5/15 |       |                |       |                 |
| 12213 | 2010/5/17 |       |                |       |                 |
| 12048 | 2010/5/23 | 674.9 | 2010_5_23_6_15 | 674.9 | 2010_5_23_6_15  |
| 12049 | 2010/5/28 |       |                |       |                 |
| 12050 | 2010/6/3  |       |                |       |                 |
| 12222 | 2010/6/5  |       |                |       |                 |
| 12219 | 2010/6/6  |       |                |       |                 |
| 12051 | 2010/6/10 |       |                |       |                 |
| 12218 | 2010/6/11 |       |                |       |                 |
| 12223 | 2010/6/13 |       |                |       |                 |
| 12052 | 2010/6/15 |       |                |       |                 |
| 12220 | 2010/6/18 | 324.6 | 2010_6_18_7_16 | 406.6 | 2010_6_18_7_22  |
| 12053 | 2010/7/5  |       |                |       |                 |
| 12054 | 2010/7/9  |       |                |       |                 |
| 12230 | 2010/7/11 |       |                |       |                 |
| 12231 | 2010/7/12 |       |                |       |                 |
| 12227 | 2010/7/14 |       |                |       |                 |
| 12233 | 2010/7/16 |       |                |       |                 |
| 12232 | 2010/7/18 | 82.0  | 2010_7_18_22   |       |                 |
| 12234 | 2010/7/22 |       |                |       |                 |
| 16183 | 2014/6/9  | 144.8 | 2014_6_09_22   | 764.7 | 2014_6_09_10_08 |
| 16180 | 2014/6/22 |       |                |       |                 |
| 16456 | 2014/7/29 | 183.3 | 2014_7_29_8_06 |       |                 |
| 16641 | 2014/7/31 |       |                |       |                 |
| 16457 | 2014/8/5  |       |                |       |                 |
| 16644 | 2014/8/6  |       |                |       |                 |

**Table S1 continued from previous page**

|       |            |       |                      |        |                      |
|-------|------------|-------|----------------------|--------|----------------------|
| 16463 | 2014/9/23  | 312.7 | 2014.9.23.10.07      |        |                      |
| 17417 | 2014/9/25  |       |                      |        |                      |
| 17416 | 2014/9/28  |       |                      |        |                      |
| 16454 | 2014/10/1  |       |                      |        |                      |
| 16176 | 2014/10/2  |       |                      |        |                      |
| 16175 | 2014/10/3  |       |                      |        |                      |
| 16178 | 2014/10/7  |       |                      |        |                      |
| 16177 | 2014/10/8  | 706.6 | 2014.10.08.11.03     |        |                      |
| 16620 | 2014/10/10 |       |                      | 1089.0 | 2014.10.10.2015.1.04 |
| 16462 | 2014/10/14 |       |                      |        |                      |
| 17535 | 2014/10/17 |       |                      |        |                      |
| 17542 | 2014/10/24 |       |                      |        |                      |
| 16184 | 2014/10/26 |       |                      |        |                      |
| 16182 | 2014/10/28 |       |                      |        |                      |
| 16181 | 2014/10/31 |       |                      |        |                      |
| 17546 | 2014/11/2  |       |                      |        |                      |
| 16186 | 2014/11/2  |       |                      |        |                      |
| 16187 | 2014/11/3  |       |                      |        |                      |
| 16188 | 2014/11/13 | 390.5 | 2014.11.13.29        |        |                      |
| 16450 | 2014/11/18 |       |                      |        |                      |
| 16190 | 2014/11/22 |       |                      |        |                      |
| 16189 | 2014/11/29 |       |                      |        |                      |
| 17556 | 2014/12/9  | 115.8 | 2014.12.09.2015.1.04 |        |                      |
| 16179 | 2014/12/31 |       |                      |        |                      |
| 17573 | 2015/1/4   |       |                      |        |                      |
| 17633 | 2015/3/16  | 226.2 | 2015.3.16.24         | 35.5   | 2015.3.16            |
| 17634 | 2015/3/19  |       |                      | 991.3  | 2015.3.19.2016.3.24  |
| 16453 | 2015/3/21  |       |                      |        |                      |
| 16451 | 2015/3/24  |       |                      |        |                      |
| 16461 | 2015/5/19  | 210.8 | 2015.5.19.25         |        |                      |
| 16191 | 2015/5/25  |       |                      |        |                      |
| 16460 | 2015/6/16  | 93.6  | 2015.6.16.20         |        |                      |
| 16459 | 2015/6/20  |       |                      |        |                      |
| 17552 | 2015/10/10 | 231.4 | 2015.10.10.30        |        |                      |

**Table S1 continued from previous page**

|            |            |       |               |      |           |  |
|------------|------------|-------|---------------|------|-----------|--|
| 16455      | 2015/10/27 |       |               |      |           |  |
| 16458      | 2015/10/30 |       |               |      |           |  |
| 17677      | 2015/11/15 | 125.1 | 2015_11_15_22 |      |           |  |
| 18709      | 2015/11/22 |       |               |      |           |  |
| 18719      | 2015/12/10 | 62.2  | 2015_12_10_12 |      |           |  |
| 16452      | 2015/12/12 |       |               |      |           |  |
| 18730      | 2016/2/2   | 29.1  | 2016_2_02     |      |           |  |
| 16185      | 2016/3/24  | 48.4  | 2016_3_24     |      |           |  |
| 0827220901 | 2019/8/6   | 29.8  | 2019_8_06     | 29.8 | 2019_8_06 |  |

**Table S2: ROSAT and Swift Observations**

| Observation ID |             | Total Exp. | Bin Name       |
|----------------|-------------|------------|----------------|
|                |             | (ks)       |                |
| ROSAT          | Swift       |            |                |
| RP190479N00    |             | 8.2        | 1997           |
| RP190075N00    |             |            |                |
| RP190477N00    |             |            |                |
|                | 00037172001 | 41.5       | 2007_7_07_8_10 |
|                | 00037172002 |            |                |
|                | 00037172003 |            |                |
|                | 00037172004 |            |                |
|                | 00037172005 |            |                |
|                | 00037172008 |            |                |

**Table S2 continued from previous page**

|             |       |                  |
|-------------|-------|------------------|
| 00037172009 |       |                  |
| 00037172010 |       |                  |
| 00037172011 |       |                  |
| 00037172012 |       |                  |
| 00037172015 |       |                  |
| 00037172016 |       |                  |
| 00037172017 |       |                  |
| 00037172018 |       |                  |
| 00037172019 |       |                  |
| 00037172021 |       |                  |
| 00037172022 |       |                  |
| 00037172023 |       |                  |
| 00037172024 |       |                  |
| 00037172025 |       |                  |
| 00037172026 |       |                  |
| 00037172027 |       |                  |
| 00037172028 |       |                  |
| 00037172029 |       |                  |
| 00037172030 |       |                  |
| 00037172031 |       |                  |
| 00037172037 | 107.1 | 2007_10_25_11_23 |
| 00037172038 |       |                  |

**Table S2 continued from previous page**

|             |       |               |
|-------------|-------|---------------|
| 00037172039 |       |               |
| 00037172040 |       |               |
| 00037172041 |       |               |
| 00037172043 |       |               |
| 00037172044 |       |               |
| 00037172045 |       |               |
| 00037172046 |       |               |
| 00037172047 |       |               |
| 00037172048 |       |               |
| 00037172049 |       |               |
| 00037172050 |       |               |
| 00037172051 |       |               |
| 00037172052 |       |               |
| 00037172053 |       |               |
| 00037172054 |       |               |
| 00037172055 |       |               |
| 00037172056 |       |               |
| 00037172057 |       |               |
| 00037172058 |       |               |
| 00037172059 |       |               |
| 00037172060 |       |               |
| 00037172061 | 383.5 | 2007_11_24_29 |

**Table S2 continued from previous page**

00037172062

00037172063

00037172064

00037172065

00037172066

00037172067

00037172068

00037172069

00037172070

00037172071

00037172072

00037172073

00037172074

00037172075

00037172076

00037172077

00037172079

00037172080

00037172081

00037172082

00037172083

00037172084

**Table S2 continued from previous page**

00037172085

00037172086

00037172087

00037172088

00037172089

00037172090

---

Table S3: The detection results of various time bins

| bin name             | LRT significance |       |       | net counts              |                         |                        | zpow.index          | ztbabs.nH                 |
|----------------------|------------------|-------|-------|-------------------------|-------------------------|------------------------|---------------------|---------------------------|
|                      | $\sigma$         |       |       |                         |                         |                        |                     | $10^{22} \text{ cm}^{-2}$ |
|                      | full             | soft  | hard  | full                    | soft                    | hard                   |                     |                           |
|                      | (1)              | (2)   | (3)   | (4)                     | (5)                     | (6)                    | (7)                 | (8)                       |
| <b>1999_10</b>       | 14.78            | 14.21 | 6.02  | $61.3^{+8.5}_{-8.4}$    | $46.6^{+7.6}_{-7.0}$    | $14.8^{+19.4}_{-10.8}$ |                     |                           |
| <b>1999_11</b>       | 19.74            | 19.86 | 6.67  | $107.2^{+11.2}_{-11.1}$ | $87.0^{+9.9}_{-9.8}$    | $20.1^{+25.6}_{-15.4}$ | $2.1^{+0.2}_{-0.2}$ | $< 0.086$                 |
| <b>2000_5_6</b>      | 19.01            | 20.31 | 5.64  | $131.1^{+12.6}_{-12.5}$ | $108.0^{+11.1}_{-11.0}$ | $23.1^{+29.4}_{-17.5}$ | $2.5^{+0.4}_{-0.4}$ | $0.16^{+0.16}_{-0.14}$    |
| <b>2000_12</b>       | 28.23            | 27.09 | 12.34 | $308.4^{+19.6}_{-19.4}$ | $221.1^{+16.2}_{-16.0}$ | $87.4^{+98.4}_{-76.4}$ | $1.8^{+0.1}_{-0.1}$ | $< 0.075$                 |
| <b>2001_7</b>        | 3.96             | 4.54  | 0.60  | $42.1^{+13.1}_{-12.1}$  | $38.3^{+11.0}_{-10.2}$  | $3.8^{+9.8}_{-0.0}$    |                     |                           |
| <b>2002_1_13_23</b>  | 4.59             | 6.33  | -0.22 | $105.2^{+25.2}_{-25.0}$ | $109.0^{+20.3}_{-20.1}$ | $0.0^{+14.5}_{-0.0}$   | $3.2^{+1.5}_{-0.9}$ | $0.26^{+0.37}_{-0.24}$    |
| <b>2004_11</b>       | 8.71             | 10.36 | 2.54  | $48.7^{+8.8}_{-8.1}$    | $38.5^{+7.2}_{-6.5}$    | $10.2^{+15.5}_{-5.7}$  |                     |                           |
| <b>2007_9_20</b>     | 0.88             | 1.89  | -0.32 | $1.9^{+2.4}_{-1.9}$     | $2.5^{+2.3}_{-1.6}$     | $0.0^{+2.2}_{-0.0}$    |                     |                           |
| <b>2007_9_22</b>     | 3.04             | 3.81  | 0.91  | $7.7^{+3.9}_{-3.2}$     | $6.0^{+3.1}_{-2.4}$     | $1.8^{+4.0}_{-0.0}$    |                     |                           |
| <b>2007_10_03_30</b> | 1.56             | 3.40  | -0.63 | $11.4^{+7.7}_{-7.0}$    | $15.1^{+5.9}_{-5.2}$    | $0.0^{+5.0}_{-0.0}$    |                     |                           |

Table S3 continued from previous page

|                       |      |       |       |                         |                         |                        |                     |        |
|-----------------------|------|-------|-------|-------------------------|-------------------------|------------------------|---------------------|--------|
| <b>2007_11_01</b>     | 3.22 | 2.98  | 1.85  | $12.1^{+5.2}_{-4.5}$    | $6.5^{+3.6}_{-2.8}$     | $5.7^{+9.6}_{-2.4}$    |                     |        |
| <b>2007_11_04</b>     | 1.03 | 0.79  | 0.72  | $3.3^{+3.3}_{-2.8}$     | $1.3^{+2.1}_{-1.3}$     | $2.0^{+4.7}_{-0.0}$    |                     |        |
| <b>2008_7_05_11</b>   | 4.81 | 4.89  | 1.65  | $178.0^{+39.4}_{-39.1}$ | $136.1^{+30.2}_{-30.1}$ | $40.2^{+64.3}_{-17.1}$ | $2.2^{+0.9}_{-0.4}$ | < 0.32 |
| <b>2009_1_06_16</b>   | 1.97 | 2.72  | 0.05  | $55.6^{+28.2}_{-27.9}$  | $54.9^{+21.2}_{-21.4}$  | $0.9^{+21.1}_{-0.0}$   |                     |        |
| <b>2009_1_18_22</b>   | 5.78 | 5.62  | 2.60  | $131.4^{+25.6}_{-25.4}$ | $89.4^{+18.5}_{-18.6}$  | $42.2^{+60.1}_{-25.2}$ | $1.2^{+0.6}_{-0.2}$ | < 0.27 |
| <b>2009_1_24</b>      | 2.73 | 1.87  | 1.98  | $45.0^{+18.2}_{-17.3}$  | $21.6^{+12.4}_{-11.6}$  | $23.4^{+36.4}_{-11.5}$ |                     |        |
| <b>2009_7_05</b>      | 2.67 | 3.37  | 0.36  | $45.5^{+18.7}_{-17.8}$  | $41.4^{+14.5}_{-13.4}$  | $4.2^{+15.0}_{-0.0}$   |                     |        |
| <b>2009_7_17</b>      | 4.37 | 3.25  | 2.93  | $83.7^{+21.3}_{-21.1}$  | $45.9^{+16.2}_{-15.3}$  | $37.9^{+52.7}_{-24.0}$ |                     |        |
| <b>2009_7_27_29</b>   | 2.69 | 2.83  | 1.01  | $65.5^{+25.5}_{-25.4}$  | $47.9^{+18.7}_{-17.8}$  | $17.7^{+32.7}_{-3.4}$  |                     |        |
| <b>2010_1_04_19</b>   | 0.53 | -0.50 | 1.25  | $13.8^{+20.9}_{-13.8}$  | $0.0^{+15.2}_{-0.0}$    | $23.2^{+40.3}_{-6.9}$  |                     |        |
| <b>2010_1_26_2_05</b> | 5.47 | 5.79  | 1.92  | $120.3^{+24.6}_{-24.6}$ | $90.6^{+18.3}_{-18.5}$  | $29.6^{+45.9}_{-14.3}$ | $1.8^{+0.6}_{-0.5}$ | < 0.12 |
| <b>2010_2_11_17</b>   | 0.93 | 0.98  | 0.34  | $22.9^{+20.2}_{-19.4}$  | $17.0^{+14.8}_{-14.0}$  | $5.9^{+21.6}_{-0.0}$   |                     |        |
| <b>2010_3_18_5_17</b> | 2.06 | 3.00  | 0.40  | $20.0^{+10.5}_{-9.8}$   | $16.8^{+7.0}_{-6.3}$    | $3.2^{+10.4}_{-0.0}$   |                     |        |
| <b>2010_5_23_6_15</b> | 1.99 | 3.94  | -0.45 | $16.8^{+9.3}_{-8.5}$    | $19.8^{+6.7}_{-6.0}$    | $0.0^{+6.1}_{-0.0}$    |                     |        |
| <b>2010_6_18_7_22</b> | 1.40 | 3.33  | -0.85 | $8.8^{+6.4}_{-5.9}$     | $12.9^{+5.3}_{-4.7}$    | $0.0^{+3.9}_{-0.0}$    |                     |        |

---

**Table S3 continued from previous page**

|                             |       |       |       |                      |                      |                      |
|-----------------------------|-------|-------|-------|----------------------|----------------------|----------------------|
| <b>2014_6_09_10_08</b>      | 1.75  | 3.42  | -0.34 | $12.8^{+7.9}_{-7.3}$ | $14.8^{+5.8}_{-5.2}$ | $0.0^{+5.7}_{-0.0}$  |
| <b>2014_10_10_2015_1_04</b> | 0.07  | -0.27 | 0.25  | $0.6^{+8.5}_{-0.6}$  | $0.0^{+4.5}_{-0.0}$  | $1.7^{+8.5}_{-0.0}$  |
| <b>2015_3_16</b>            | 3.16  | 0.72  | 3.13  | $7.4^{+3.7}_{-3.1}$  | $0.6^{+1.6}_{-0.6}$  | $6.8^{+10.3}_{-3.9}$ |
| <b>2015_3_19_2016_3_24</b>  | 1.18  | 0.05  | 1.35  | $9.9^{+7.9}_{-7.3}$  | $0.2^{+5.0}_{-0.2}$  | $9.7^{+16.8}_{-3.1}$ |
| <b>2019_8</b>               | -0.23 | -0.11 | -0.21 | $0.0^{+7.2}_{-0.0}$  | $0.0^{+5.5}_{-0.0}$  | $0.0^{+5.6}_{-0.0}$  |

---

Table S4: Adaptive-bin Results

| Bin Name         | Time         | Lumin <sub>0.5–7.0 keV</sub>            | Lumin <sub>0.5–2.0 keV</sub>            |
|------------------|--------------|-----------------------------------------|-----------------------------------------|
|                  | MJD          | erg s <sup>-1</sup>                     | erg s <sup>-1</sup>                     |
| (1)              | (2)          | (3)                                     | (4)                                     |
| 1997             | 50491.5±5.0  | none                                    | < 42.44                                 |
| 1999_10          | 51466.5±0.6  | 42.30 <sup>+0.06</sup> <sub>-0.06</sub> | 42.06 <sup>+0.07</sup> <sub>-0.07</sub> |
| 1999_11          | 51505.7±0.6  | 42.40 <sup>+0.04</sup> <sub>-0.05</sub> | 42.19 <sup>+0.05</sup> <sub>-0.05</sub> |
| 2000_5_6         | 51695.4±4.3  | 42.27 <sup>+0.04</sup> <sub>-0.04</sub> | 42.07 <sup>+0.04</sup> <sub>-0.05</sub> |
| 2000_12          | 51896.1±7.1  | 42.12 <sup>+0.03</sup> <sub>-0.03</sub> | 41.86 <sup>+0.03</sup> <sub>-0.03</sub> |
| 2001_7           | 52118.1±0.6  | 41.85 <sup>+0.12</sup> <sub>-0.15</sub> | 41.68 <sup>+0.11</sup> <sub>-0.13</sub> |
| 2002_1_13_23     | 52292.8±5.2  | 41.50 <sup>+0.09</sup> <sub>-0.12</sub> | 41.39 <sup>+0.07</sup> <sub>-0.09</sub> |
| 2004_11          | 53326.4±4.3  | 41.87 <sup>+0.07</sup> <sub>-0.08</sub> | 41.67 <sup>+0.07</sup> <sub>-0.08</sub> |
| 2007_7_07_8_10   | 54305.2±16.5 | < 42.22                                 | < 41.98                                 |
| 2007_9_20        | 54363.5±0.3  | < 41.85                                 | < 41.74                                 |
| 2007_9_22        | 54366.1±0.3  | 41.98 <sup>+0.18</sup> <sub>-0.24</sub> | 41.77 <sup>+0.18</sup> <sub>-0.23</sub> |
| 2007_10_03_30    | 54390.5±13.9 | < 41.24                                 | 40.95 <sup>+0.14</sup> <sub>-0.19</sub> |
| 2007_11_01       | 54406.3±0.8  | 41.41 <sup>+0.16</sup> <sub>-0.20</sub> | < 41.33                                 |
| 2007_11_04       | 54408.8±0.7  | < 41.76                                 | < 41.43                                 |
| 2007_10_25_11_23 | 54412.7±14.6 | < 41.99                                 | < 41.83                                 |
| 2007_11_24_29    | 54446.4±17.6 | < 41.71                                 | < 41.74                                 |
| 2008_7_05_11     | 54655.9±3.7  | 41.57 <sup>+0.09</sup> <sub>-0.11</sub> | 41.33 <sup>+0.09</sup> <sub>-0.11</sub> |
| 2009_1_06_16     | 54843.5±5.6  | < 41.53                                 | < 41.37                                 |

**Table S4 continued from previous page**

|                      |               |                                         |                                         |
|----------------------|---------------|-----------------------------------------|-----------------------------------------|
| 2009_1_18_22         | 54852.5±2.7   | 41.82 <sup>+0.08</sup> <sub>-0.09</sub> | 41.53 <sup>+0.08</sup> <sub>-0.10</sub> |
| 2009_1_24            | 54856.5±0.7   | < 41.87                                 | < 41.49                                 |
| 2009_7_05            | 55018.1±0.7   | < 41.77                                 | 41.39 <sup>+0.13</sup> <sub>-0.17</sub> |
| 2009_7_17            | 55030.0±0.7   | 41.88 <sup>+0.10</sup> <sub>-0.13</sub> | 41.50 <sup>+0.13</sup> <sub>-0.18</sub> |
| 2009_7_27_29         | 55040.9±1.8   | < 41.62                                 | < 41.37                                 |
| 2010_1_04_19         | 55208.5±7.7   | < 41.34                                 | < 40.91                                 |
| 2010_1_26_2_05       | 55228.4±5.7   | 41.80 <sup>+0.08</sup> <sub>-0.10</sub> | 41.56 <sup>+0.08</sup> <sub>-0.10</sub> |
| 2010_2_11_17         | 55242.4±3.7   | < 41.35                                 | < 41.09                                 |
| 2010_3_18_5_17       | 55303.7±30.6  | < 41.33                                 | 40.89 <sup>+0.15</sup> <sub>-0.20</sub> |
| 2010_5_23_6_15       | 55351.6±12.3  | < 41.37                                 | 41.08 <sup>+0.13</sup> <sub>-0.16</sub> |
| 2010_6_18_7_22       | 55383.0±17.4  | < 41.33                                 | 41.06 <sup>+0.15</sup> <sub>-0.19</sub> |
| 2014_6_09_10_08      | 56879.0±61.4  | < 41.32                                 | 41.01 <sup>+0.14</sup> <sub>-0.19</sub> |
| 2014_10_10_2015_1_04 | 56983.6±43.1  | < 40.87                                 | < 40.52                                 |
| 2015_3_16            | 57097.8±0.2   | 42.31 <sup>+0.18</sup> <sub>-0.23</sub> | < 42.01                                 |
| 2015_3_19_2016_3_24  | 57286.1±185.9 | < 41.26                                 | < 40.80                                 |
| 2019_8               | 58701.8±0.2   | < 41.83                                 | < 41.58                                 |

- 
1. Column 1: name of the time bin.
  2. Column 2: time of each time bin.
  3. Column 3: 0.5–7.0 keV (rest-frame) luminosity. The value without error is 90% confidence level upper limit.
  4. Column 4: same as Column 3, but for luminosity in 0.5–2.0 keV (rest-frame).

Table S5: One-month-bin Results

| Bin Name         | Time         | Lumin <sub>0.5–7.0 keV</sub>            | Lumin <sub>0.5–2.0 keV</sub>            |
|------------------|--------------|-----------------------------------------|-----------------------------------------|
|                  | MJD          | erg s <sup>-1</sup>                     | erg s <sup>-1</sup>                     |
| (1)              | (2)          | (3)                                     | (4)                                     |
| 1997             | 50491.5±5.0  | none                                    | < 42.44                                 |
| 1999_10          | 51466.5±0.6  | 42.30 <sup>+0.06</sup> <sub>-0.06</sub> | 42.06 <sup>+0.07</sup> <sub>-0.07</sub> |
| 1999_11          | 51505.7±0.6  | 42.40 <sup>+0.04</sup> <sub>-0.05</sub> | 42.19 <sup>+0.05</sup> <sub>-0.05</sub> |
| 2000_5_6         | 51695.4±4.3  | 42.27 <sup>+0.04</sup> <sub>-0.04</sub> | 42.07 <sup>+0.04</sup> <sub>-0.05</sub> |
| 2000_12          | 51896.1±7.1  | 42.12 <sup>+0.03</sup> <sub>-0.03</sub> | 41.86 <sup>+0.03</sup> <sub>-0.03</sub> |
| 2001_7           | 52118.1±0.6  | 41.85 <sup>+0.12</sup> <sub>-0.15</sub> | 41.68 <sup>+0.11</sup> <sub>-0.13</sub> |
| 2002_1           | 52292.8±5.2  | 41.50 <sup>+0.09</sup> <sub>-0.12</sub> | 41.39 <sup>+0.07</sup> <sub>-0.09</sub> |
| 2004_11          | 53326.4±4.3  | 41.87 <sup>+0.07</sup> <sub>-0.08</sub> | 41.67 <sup>+0.07</sup> <sub>-0.08</sub> |
| 2007_7_07_8_10   | 54305.2±16.5 | < 42.22                                 | < 41.98                                 |
| 2007_9_20_10_19  | 54378.6±15.4 | 41.43 <sup>+0.14</sup> <sub>-0.18</sub> | 41.26 <sup>+0.12</sup> <sub>-0.15</sub> |
| 2007_10_22_11_04 | 54402.5±7.0  | < 41.33                                 | 40.90 <sup>+0.15</sup> <sub>-0.19</sub> |
| 2007_10_25_11_23 | 54412.7±14.6 | < 41.99                                 | < 41.83                                 |
| 2007_11_24_29    | 54446.4±17.6 | < 41.71                                 | < 41.74                                 |
| 2008_7           | 54655.9±3.7  | 41.57 <sup>+0.09</sup> <sub>-0.11</sub> | 41.33 <sup>+0.09</sup> <sub>-0.11</sub> |
| 2009_1_06_24     | 54847.6±9.7  | 41.59 <sup>+0.07</sup> <sub>-0.09</sub> | 41.33 <sup>+0.07</sup> <sub>-0.09</sub> |
| 2009_7_05_29     | 55030.0±12.7 | 41.59 <sup>+0.08</sup> <sub>-0.09</sub> | 41.31 <sup>+0.08</sup> <sub>-0.10</sub> |
| 2010_1_04_26     | 55212.5±11.7 | < 41.56                                 | < 41.26                                 |
| 2010_2_05_17     | 55239.4±6.7  | < 41.56                                 | < 41.27                                 |

**Table S5 continued from previous page**

|                      |              |         |                                         |
|----------------------|--------------|---------|-----------------------------------------|
| 2010_3_18_4_16       | 55288.3±15.2 | < 41.31 | < 41.13                                 |
| 2010_4_18_5_17       | 55319.4±14.9 | < 41.57 | < 41.37                                 |
| 2010_5_23_6_15       | 55351.6±12.3 | < 41.37 | 41.08 <sup>+0.13</sup> <sub>-0.16</sub> |
| 2010_6_18_7_16       | 55379.7±14.2 | < 41.42 | < 41.34                                 |
| 2010_7_18_22         | 55398.1±2.3  | < 41.46 | < 41.44                                 |
| 2014_6_09_22         | 56824.3±6.7  | < 41.56 | < 41.48                                 |
| 2014_7_29_8_06       | 56871.9±4.0  | < 41.42 | < 41.41                                 |
| 2014_9_23_10_07      | 56930.7±7.7  | < 41.48 | < 41.18                                 |
| 2014_10_08_11_03     | 56951.8±12.9 | < 41.01 | < 40.76                                 |
| 2014_11_13_29        | 56982.7±8.6  | < 41.08 | < 40.98                                 |
| 2014_12_09_2015_1_04 | 57013.8±12.8 | < 41.63 | < 41.14                                 |
| 2015_3_16_24         | 57102.4±4.8  | < 42.00 | < 41.46                                 |
| 2015_5_19_25         | 57164.7±3.6  | < 41.34 | < 41.21                                 |
| 2015_6_16_20         | 57191.7±2.4  | < 41.70 | < 41.40                                 |
| 2015_10_10_30        | 57316.2±10.9 | < 41.59 | < 41.10                                 |
| 2015_11_15_22        | 57345.4±3.7  | < 41.75 | < 41.47                                 |
| 2015_12_10_12        | 57367.8±1.5  | < 41.53 | < 41.39                                 |
| 2016_2_02            | 57420.6±0.2  | < 41.93 | < 41.78                                 |
| 2016_3_24            | 57471.7±0.3  | < 42.18 | < 41.90                                 |
| 2019_8_06            | 58701.8±0.2  | < 41.83 | < 41.58                                 |

---

Table S6: Model Parameters for SED Fitting with CIGALE

| Module                                                                          | Parameter                         | Values                                                                         |
|---------------------------------------------------------------------------------|-----------------------------------|--------------------------------------------------------------------------------|
| Star-formation history $\text{SFR} \propto (t - T_0) \exp(-\frac{t-T_0}{\tau})$ | Stellar e-folding time            | 0.1, 0.2, 0.3, 0.4, 0.5, 0.6, 0.7, 0.8, 0.9, 1, 2, 3, 4, 5, 6, 7, 8, 9, 10 Gyr |
|                                                                                 | Stellar age                       | 0.1, 0.2, 0.3, 0.4, 0.5, 0.6, 0.7, 0.8, 0.9, 1, 2, 3, 4, 5, 6, 7, 8, 9, 10 Gyr |
| Simple stellar population                                                       | Initial mass function             | Chabrier                                                                       |
|                                                                                 | Metallicity                       | 0.0001, 0.0004, 0.004, 0.008, 0.02, 0.05                                       |
| Dust attenuation                                                                | $E(B - V)_{\text{line}}$          | 0, 0.05, 0.1, 0.15, 0.2, 0.25, 0.3, 0.4, 0.5,                                  |
|                                                                                 |                                   | 0.6, 0.7, 0.8, 0.9, 1, 1.2, 1.5                                                |
| Galactic dust emission                                                          | Slope in $dU/dM \propto U^\alpha$ | 1.0, 1.5, 2.0, 2.5, 3.0                                                        |

**Note.** For parameters not listed here, we use the default values.
